# Supplementary material for: Mixed quantum-classical dynamics using collective electronic variables: A better alternative to electronic friction theories
Source: arXiv:1611.06525 ancillary file (2016-11-20)
Supplement: Supplementary file 1 [file fric_supp.pdf]

## Supplementary information

### I. INTEGRATION OF THE FRICTION KERNEL

The right-hand side of the Langevin equation (Eq. 7 of the main text) can be conveniently rewritten as

$$G^\alpha(t) = -2\hbar \sum_{k>0} g_{k0}^\alpha(t) e_k(t), \quad (1)$$

where  $g_{k0}^\alpha(t) = f_{k0}^\alpha(t)/\omega_{k0}$  are the derivative non-adiabatic couplings and

$$e_k(t) = \int_0^t \tau_{k0}(t') \omega_{k0} \cos(\omega_{k0} \times (t - t')) dt'. \quad (2)$$

We have also used the identity  $\sum_\beta g_{k0}^\beta(t') \dot{R}_\beta(t') = \tau_{k0}(t')$ . The time derivative of  $e_k(t)$  is:

$$\dot{e}_k(t) = \tau_{k0}(t) \omega_{k0} - \omega_{k0} \int_0^t \tau_{k0}(t') \omega_{k0} \sin(\omega_{k0} \times (t - t')) dt'. \quad (3)$$

It is natural to introduce additional variables

$$f_k(t) = \int_0^t \tau_{k0}(t') \omega_{k0} \sin(\omega_{k0} \times (t - t')) dt' \quad (4)$$

and the corresponding equations of motion (EOM)

$$\dot{f}_k(t) = \omega_{k0} \int_0^t \tau_{k0}(t') \omega_{k0} \cos(\omega_{k0} \times (t - t')) dt' = \omega_{k0} e_k(t). \quad (5)$$

Eqs. (3) and (5) describe dynamics of driven harmonic oscillators, each of those vibrates with the frequency  $\omega_{k0}$ . We integrate them numerically to obtain  $G^\alpha(t)$ , which is subsequently used for solving the Langevin equation. We note in the passing that the very form of Eqs. (3) and (5) confirms the representation of the electronic subsystem as a collection of harmonic oscillators that are linearly coupled to the nuclear subsystem through the term (1).

### II. COLLECTIVE VARIABLE TRANSFORMATION

#### A. Two collective mode (2CM) model

With our second major assumption, namely,

$$\tau_{kj} = 0, \quad k, j \geq 1, \quad (6)$$

the interaction matrix  $\mathbf{T}$  assumes the form

$$\mathbf{T} = \begin{pmatrix} 0 & -\tau_{10}e^{-i\phi_{10}} & \dots & -\tau_{n0}e^{i\phi_{n0}} \\ \tau_{10}e^{i\phi_{10}} & 0 & \dots & 0 \\ \vdots & \vdots & \ddots & \vdots \\ \tau_{n0}e^{i\phi_{n0}} & 0 & \dots & 0 \end{pmatrix}. \quad (7)$$

It can be block-diagonalized by a similarity transformation  $\mathbf{Z} = \mathbf{U}^{-1}\mathbf{T}\mathbf{U}$  with

$$\begin{aligned} \mathbf{U} &= \text{diag}\{1, e^{i\phi_{10}}, \dots, e^{i\phi_{1n}}\} \\ &\times z^{-1} \begin{pmatrix} 1 & 0 & 0 & \dots & 0 \\ 0 & \tau_{10} & \tau_{20} & \dots & \tau_{n0} \\ 0 & \tau_{20} & -\tau_{10} & \dots & 0 \\ \vdots & \vdots & & \ddots & \\ 0 & \tau_{n0} & 0 & \dots & -\tau_{10} \end{pmatrix}, \end{aligned} \quad (8)$$

where  $z = (\sum_{k=1}^n \tau_{k0}^2)^{1/2}$ .

### B. Three collective mode (3CM) model

If time-derivatives of the ratios

$$p_k = \frac{\tau_{k0}}{\tau_{10}}, \quad k > 1 \quad (9)$$

are small:

$$\dot{p}_k \ll 1, \quad k > 1, \quad (10)$$

then  $\mathbf{N} = \mathbf{U}^{-1} \dot{\mathbf{U}}$  is approximated as

$$\mathbf{N} \approx i \text{diag} \{0, \tilde{w}_{11}, \tilde{w}_{22}, \dots, \tilde{w}_{nn}\} - i \frac{\tau_{10}^2}{z^2} \begin{pmatrix} 0 & 0 & 0 & 0 & \cdots & 0 \\ 0 & 0 & p_2 \omega_{21} & p_3 \omega_{31} & \cdots & p_n \omega_{n1} \\ 0 & p_2 \left( \omega_{21} - \sum_{j \neq 2} p_j^2 \omega_{j2} \right) & 0 & p_2 p_3 \omega_{31} & \cdots & p_2 p_n \omega_{n1} \\ 0 & p_3 \left( \omega_{31} - \sum_{j \neq 3} p_j^2 \omega_{j3} \right) & p_3 p_2 \omega_{21} & 0 & \cdots & p_3 p_n \omega_{n1} \\ \vdots & \vdots & \vdots & \vdots & \ddots & \vdots \\ 0 & p_n \left( \omega_{n1} - \sum_{j \neq n} p_j^2 \omega_{jn} \right) & p_n p_2 \omega_{21} & p_n p_3 \omega_{31} & \cdots & 0 \end{pmatrix}, \quad (11)$$

where

$$\tilde{w}_{kk} = w_{k0} - \frac{\tau_{k0}^2}{z^2} \omega_{k1}, \quad k > 1. \quad (12)$$

Keeping (in the spirit of the perturbation theory) only zero and first powers of  $p_k$  on off-diagonals, we obtain a properly anti-Hermitian  $\mathbf{N}^{(a)}$ :

$$\mathbf{N}^{(a)} = i \text{diag} \{0, \tilde{w}_{11}, \tilde{w}_{22}, \dots, \tilde{w}_{nn}\} - i \begin{pmatrix} 0 & 0 & 0 & \cdots & 0 \\ 0 & 0 & \pi_2 & \cdots & \pi_n \\ 0 & \pi_2 & 0 & \cdots & 0 \\ \vdots & \vdots & \vdots & \ddots & \vdots \\ 0 & \pi_n & 0 & \cdots & 0 \end{pmatrix}, \quad (13)$$

where

$$\pi_k = p_k \frac{\tau_{10}^2}{z^2} \omega_{k1}, \quad k > 1. \quad (14)$$

### III. MOLECULAR MODEL: AN ATOM ON A METALLIC CHAIN

We parametrize the electronic Hamiltonian  $\hat{H}_e$  in the diabatic representation as a Hermitian matrix

$$\mathbf{H}_e = \begin{pmatrix} V_{00}(R) & \cdots & V_{n0}(R) \\ \vdots & \ddots & \vdots \\ V_{n0}(R) & \cdots & V_{nn}(R) \end{pmatrix} \quad (15)$$

with matrix elements that are constants or polynomials in  $R$ . Diagonalization of  $\mathbf{H}_e$  determines the adiabatic potentials  $\{E_k(R)\}$  and the corresponding non-adiabatic forces  $\{f_{kj}(R)\}$  and couplings  $\{\tau_{kj}\}$ .

We begin with a pair parabolic potential  $V(R)$ , which describes chemical bonding in an adatom-metal dimer AMe:

$$V(R) = \frac{M\Omega^2 R^2}{2}, \quad (16)$$

TABLE I. Parameters of an adatom-metal chain model (in atomic units) used to generate the results for Fig. 2 of the main text.

| Parameter                               | Value                          |
|-----------------------------------------|--------------------------------|
| Number of Me atoms in a chain, $2n + 1$ | 9                              |
| States per layer, $m + 1$               | 1, 5, and 10                   |
| Adatom mass, $M$                        | 2000                           |
| Harmonic frequency, $\Omega$            | 0.0028 (614 cm <sup>-1</sup> ) |
| Me–Me distance, $D$                     | 5.0 (2.645 Å)                  |
| Inter-layer couplings:                  |                                |
| $\beta$                                 | 0.03                           |
| $\gamma$                                | 0.02                           |
| $\delta$ and higher                     | 0.01                           |
| Intra-layer offset, $d$                 | $1.0 \times 10^{-4}$           |
| Intra-layer coupling, $\alpha$          | 0.004                          |

where  $\Omega$  is a harmonic frequency.

The pair potential is the main building block in a model, where  $(2n + 1)$  displaced potentials

$$V_{kD}(R) = V(R - kD), \quad -n \leq k \leq n \quad (17)$$

are coupled in a potential matrix

$$V^{\text{mol}}(R) = \begin{pmatrix} V_{-nD}(R) & \beta & \gamma & \cdots \\ \beta & V_{(-n+1)D}(R) & \beta & \vdots \\ \vdots & \beta & \ddots & \\ \cdots & \cdots & & V_{nD}(R) \end{pmatrix} \quad (18)$$

through constants  $\beta, \gamma, \dots$ .  $D$  is a distance between Me atoms in a chain.  $\Omega, \beta, \gamma, \dots$ , and  $D$  together determine barrier heights for translation of an adatom from one metallic center to another.  $(2n + 1)D$  is the total length of the chain, which has to be large enough to allow for dynamics free from edge effects.

The diabatic model with  $V^{\text{mol}}(R)$  taken as  $\mathbf{H}_e$  describes an atom on an insulator-like surface. To represent a metallic surface we need layers of virtually parallel electronic levels that correspond to modulation of A–Me interaction due to the presence of electron-hole pairs. We create such levels by cloning every single pair potential  $V_{kD}(R)$  in  $(m + 1)$  instances with small shifts  $ld$ ,  $0 \leq l \leq m$ , with respect to the reference position  $kD$ , where  $d$  is the small number.  $(m + 1)$  clones are coupled diabatically through a nearest-neighbour coupling constant  $\alpha \ll \beta, \gamma, \dots$  see Table I. As a result, each scalar potential  $V_{kD}(R)$  is replaced by a  $(m + 1) \times (m + 1)$  matrix

$$\mathbb{V}_{kDd\alpha}(R) = \begin{pmatrix} V_{kD}(R) & \alpha & 0 & \cdots & 0 \\ \alpha & V_{kD}(R + d) & \alpha & & \\ 0 & \alpha & V_{kD}(R + 2d) & & 0 \\ \vdots & 0 & & \ddots & \\ 0 & 0 & \cdots & & V_{kD}(R + md) \end{pmatrix}. \quad (19)$$

Each coupling constant  $\beta, \gamma$ , *etc.* becomes, in turn, a diagonal  $(m + 1) \times (m + 1)$  matrix. Overall, the total electronic Hamiltonian matrix has the same structure as  $V^{\text{mol}}(R)$ , Eq. (18), but with  $(m + 1) \times (m + 1)$  matrix entries:

$$\mathbf{H}_e = \begin{pmatrix} \mathbb{V}_{-nDd\alpha}(R) & \beta & \cdots \\ & \beta & \\ & & \ddots \end{pmatrix}. \quad (20)$$

The nuclear kinetic energy is an  $(n + 1) \times (n + 1)$  identity matrix multiplied by a scalar factor

$$T_N = \frac{M\dot{R}^2}{2}, \quad (21)$$

where  $M$  is a reduced mass assigned to the nuclear degree of freedom (DOF).

#### IV. MOLECULAR PARAMETERS FOR FIG. 3

For explanation consult Sec III and Table I.  $m + 1 = 5$ ,  $d = 1.0 \times 10^{-5}$ ,  $\alpha = 0.001$ ,  $\beta = 0.03$ ,  $\gamma = 0.09$ ,  $\delta = 0.12$ .

## V. NUMERICAL INTEGRATION

We have used the adaptive explicit Runge–Kutta (4,5) integrator as implemented by the `ode45` routine [1] from the MATLAB [2] environment for the Ehrenfest dynamics. mixed quantum-classical (MQC) equations for other models sometimes become *stiff* thus the `ode15s` integrator applied for them. Convergence parameters for the all integrators are the same: the absolute error tolerance  $1 \times 10^{-6}$ , the relative tolerance  $5 \times 10^{-6}$ , the initial time step 6 au, and the maximum time step 18 au.

- 
- [1] L. F. Shampine and M. W. Reichelt, *SIAM J. Sci. Comput.* **18**, 1 (1997).
  - [2] MATLAB, *version 8.6.0.267246 (R2015b)* (The MathWorks Inc., Natick, Massachusetts, 2015).
